# Supplementary material for: Anomalous diffusion of phospholipids and cholesterols in a lipid bilayer and its origins
Source: arXiv:1210.5485 source file (2012-10-19)
Supplement: Supplementary file 1 [file supplementary_PRL2.pdf]

# Supplementary Material:
# Anomalous diffusion of phospholipids and cholesterols in a lipid bilayer and its origins

Jae-Hyung Jeon,[1] Hector Martinez-Seara Monne,[1] Matti Javanainen,[1] and Ralf Metzler[2,1]

[1]*Department of Physics, Tampere University of Technology, FI-33101 Tampere, Finland*
[2]*Institute for Physics & Astronomy, University of Potsdam, D-14476 Potsdam-Golm, Germany*

In this supplementary document, we provide additional figures supporting the analysis in the main text and present full mathematical descriptions of the displacement autocorrelation function and the moment ratios. Moreover, we provide detailed information on the molecular dynamics simulations.

## I. ADDITIONAL FIGURES

### A. The translational motion of the lipid layers and the relative coordinate

As previously observed in other simulations [1, 2], for finite lipid bilayer systems each monolayer of the lipid bilayer undergoes translational motion relative to the other. This phenomenon has been proposed to be an intrinsic property of biological membranes which can be actively controlled by the cell. For example, it has been suggested as an important mechanism in heterogeneous membranes to reduce the thickness mismatch [3]. This phenomenon is artificially enhanced in small planar membranes like the ones used in this work. Fig. S1A displays the $x$-component of this translational motion for the upper and lower monolayers of the pure DSPC bilayer used in our simulation. The lateral dynamics of lipids is affected by this finite size effect. To see this let us write down the two-dimensional trajectory of a lipid molecule $\mathbf{R}(t)$ in the reference frame as $\mathbf{R}(t) = \mathbf{R}_{\mathrm{CM}}(t) + \mathbf{r}(t)$, where $\mathbf{R}_{\mathrm{CM}}(t)$ is the CM trajectory of the monolayer to which the lipid belongs and $\mathbf{r}(t)$ is the motion of the lipid relative to the CM. Fig. S1B shows the lateral motion of $\mathbf{R}_{\mathrm{CM}}(t)$ and $\mathbf{r}(t)$ of a lipid molecule during simulation. Compared to the lateral dynamics of a lipid within the layer (i.e. $\mathbf{r}(t)$), the lateral fluctuation of the layer is large. Therefore the MSD of $\mathbf{R}(t)$ (where $\langle\mathbf{R}^2(t)\rangle = \langle\mathbf{R}^2_{\mathrm{CM}}(t)\rangle + \langle\mathbf{r}^2(t)\rangle$) can significantly differ from that of the lipid motion within the layer, $\langle\mathbf{r}^2(t)\rangle$. Moreover, by the free (i.e., unrestricted) diffusion of the CM, $\langle\mathbf{R}^2(t)\rangle$ becomes normal diffusion at long times irrespective of the nature of the lateral motion of the lipid. To avoid this finite size effect, we use the relative coordinate of a lipid $\mathbf{r}(t)$ in our study.

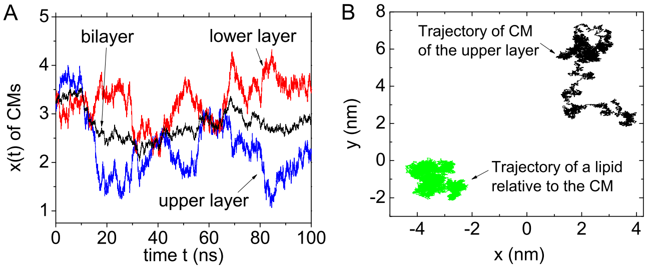


FIG. S1: (A) The $x$-component motion of CMs of the upper and lower monolayers of the pure DSPC lipid bilayer, and the CM of the bilayer. (B) Trajectory of the CM of all DSPC molecules in the upper layer $\mathbf{R}_{\mathrm{CM}}(t)$ and the lateral motion relative to the CM $\mathbf{r}(t)$ of a DSPC molecule that belongs to the upper layer.

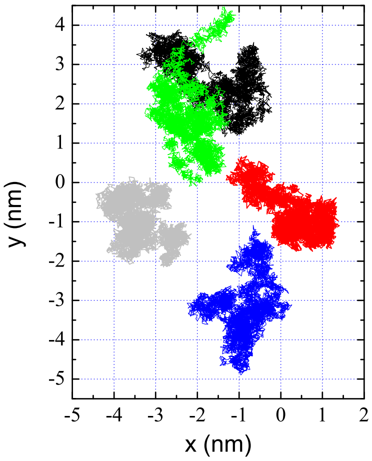


FIG. S2: Sample trajectories of the lateral motion of DSPC molecules $\mathbf{r}(t)$ relative to CM of the bilayer at 338 K. Each color corresponds to an individual lipid molecule during simulation (100 ns)

### B. Liquid disordered phase: pure phospholipid bilayer

**(1) Trajectories of DSPCs (Fig. S2)** In line with previous studies [4, 5], jump-like displacement of lipid movement is not seen in our simulation. In the liquid phase bilayer, the lateral displacement of the lipids is sufficiently large, so that some of the trajectories overlap and change of neighbors occurs (see SM I.G). Compare to the decreased mobility in presence of cholesterols (Fig. S5) and especially in the gel phase (Fig. S11).

**(2) Scatter distribution of individual TA MSDs (Fig. S3)** The scatter distributions of amplitudes between individual TA MSDs of individual trajectories are bell-shaped and become sharper as the measurement time $T$ increases, implying that the lateral diffusive process of a lipid molecule is ergodic. We use the dimensionless variable $\xi = \overline{\delta^2}/\langle\overline{\delta^2}\rangle$, where $\langle\overline{\delta^2}\rangle$ is the trajectory-to-

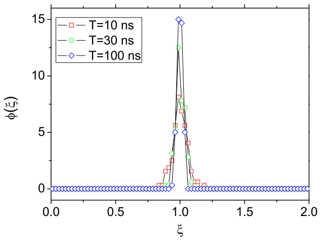


FIG. S3: Dependence of the scatter distribution $\phi(\xi)$ of trajectory-to-trajectory fluctuations of $\overline{\delta^2(\Delta, T)}$ on the measurement time $T$. Normalized scatter distributions $\phi(\xi)$ for DSPC molecules in a pure DSPC bilayer at 338 K are calculated from the TA MSDs $\overline{\delta^2}$ for three measurement times: $T = 10$ ns, 30 ns, and 100 ns, for lag time $\Delta = 0.1$ ns.

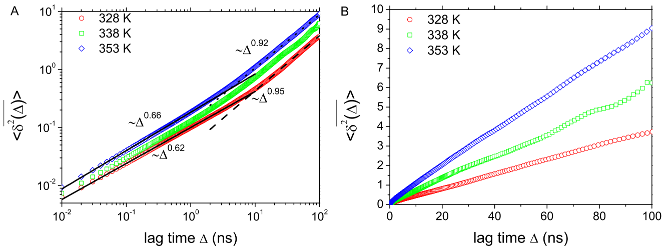


FIG. S4: Comparison of TA MSDs $\langle\overline{\delta^2(\Delta)}\rangle$, averaged over all trajectories, of DSPC molecules at different temperatures. Two additional 100 ns simulations of DSPC pure membrane at 328 K and 358 K were performed for this analysis following the same protocol described in the main paper. A. Log–log plot, the straight lines depicting the scaling behaviors at short and long times. B. Linear–linear plot of the same data.

trajectory average.

**(3) TA MSDs at different temperatures (Fig. S4)** The increase of temperature leaves the scaling exponents of the lateral diffusion virtually unaffected, while an increase of the diffusion coefficients at long times is observed.

## C. Liquid ordered phase: phospholipid bilayer with 20% cholesterol

**(1) Trajectories of DSPCs and cholesterols (Fig. S5)** In the cholesterol-containing bilayer, individual DSPC molecules exhibit lateral motions $\mathbf{r}(t)$ qualitatively similar to that of the lipids in the pure bilayer. Cholesterols also have similar lateral trajectories.

**(2) Displacement autocorrelation function (Fig. S6)** The displacement autocorrelation functions for DSPC molecules in the cholesterol-containing and the cholesterol-free bilayers are compared. They are almost identical except that the autocorrelation for the lipid with 20% mol cholesterols has a deeper well.

**(3) Moment ratios of lipids and cholesterols (Fig. S7)** The moment ratios $\langle r^4_{\max}(t)\rangle / \langle r^2_{\max}(t)\rangle^2$ (mean maximal excursion) and $\langle \mathbf{r}^4(t)\rangle / \langle \mathbf{r}^2(t)\rangle^2$ (regular) for DSPC lipids and cholesterol molecules, respectively, are plotted. In both cases the statistical behavior of the moment ratios are consistent with those of FLE motion.

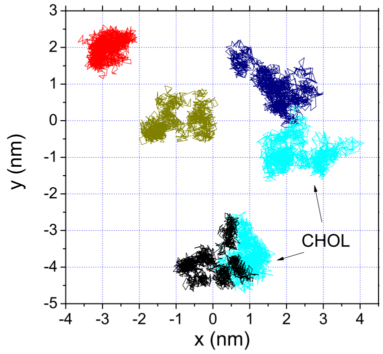


FIG. S5: Sample trajectories $\mathbf{r}(t)$ of the lateral motion of DSPC and cholesterol molecules (indicated by the arrows) during simulation (150 ns).

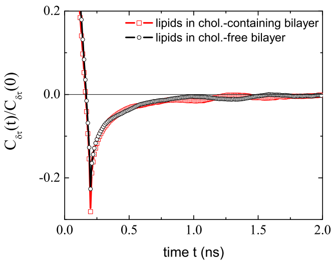


FIG. S6: Displacement autocorrelation $C_{\delta t}(t)/C_{\delta t}(0)$ for DSPC molecules in cholesterol-containing and cholesterol-free bilayers, at $\delta t = 0.2$ ns.

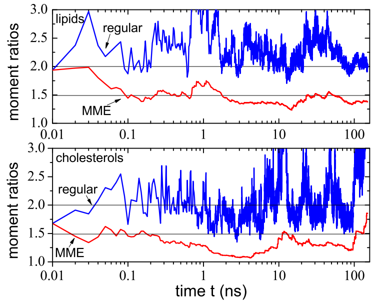


FIG. S7: Moment ratios $\langle r^4_{\max}(t)\rangle / \langle r^2_{\max}(t)\rangle^2$ (MME) and $\langle \mathbf{r}^4(t)\rangle / \langle \mathbf{r}^2(t)\rangle^2$ (regular) for DSPC lipids and cholesterols. The horizontal line at 1.49 is the critical value distinguishing FLE-like subdiffusion from CTRW-like subdiffusion for the MME moments: $\langle r^4_{\max}(t)\rangle / \langle r^2_{\max}(t)\rangle^2 < 1.49$ for FLE and $\langle r^4_{\max}(t)\rangle / \langle r^2_{\max}(t)\rangle^2 > 1.49$ for CTRW motion. The horizontal line at 2 is the theoretical value for the regular moment ratio for both FLE and CTRW motions.

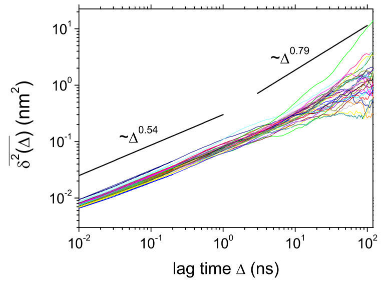


FIG. S8: $\overline{\delta^2(\Delta)}$ for the 32 cholesterols in the cholesterol-containing bilayer.

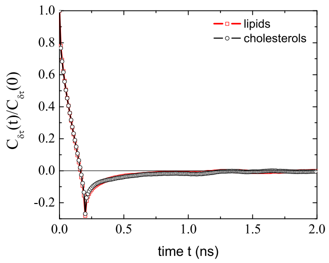


FIG. S9: Comparison of displacement autocorrelation functions of DSPC lipids and cholesterols in cholesterol-containing bilayer, with $\delta t = 0.2$ ns.

**(4) Individual TA MSDs of the cholesterols (Fig. S8)** Individual TA MSDs follow scaling behaviors (indicated by the two solid lines) for their mean TA MSD $\langle\overline{\delta^2(\Delta)}\rangle$ shown in the main text. (NB) The scatter distribution of these 32 TA MSDs is presented in Fig. 4B (main text).

**(5) Displacement autocorrelation function of cholesterols and lipids (Fig. S9)** The autocorrelation function of the cholesterols almost overlaps with that of the lipids, meaning that the lateral motion of the cholesterols follows FLE-type motion.

**(6) TA MSD of DSPCs for 1 $\mu$s-long simulation (Fig. S10)** Additional simulations of DSPC bilayer system mixed with 20% cholesterols were performed up to 1 $\mu$s. Consistent with the simulation by Flenner et al. [6], ballistic behavior of lipid motion is observed on the time scale of femtoseconds. The new simulation reproduces the consistent subdiffusive behavior of the DSPC molecules for the time window shown in Fig. 2B. Fig. S10 demonstrates that the second subdiffusion regime is, in fact, a long transition period before the Brownian regime; after the crossover time $\tau_c \approx 10$ ns the slope of the MSD curve continuously increases, eventually becoming a linear at around 400-500 ns. However, for the time windows discussed in the main text the power-law fit with the listed long-time exponents appears as a good measure.

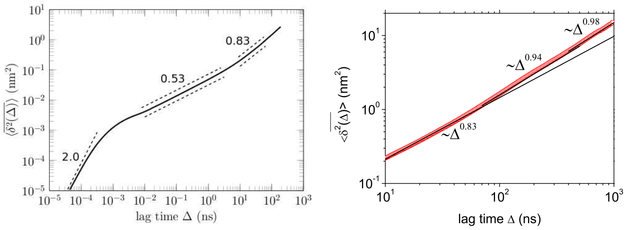


FIG. S10: TA MSD $\langle\overline{\delta^2(\Delta)}\rangle$ averaged over the trajectories of all DSPCs for the 1 $\mu$s-long simulation of a lipid bilayer with 20% cholesterol. To obtain the ballistic regime of the MSD curve, two additional simulations (i) from 0 to 100 ps saving every 1 fs and (ii) from 0 to 10 ns saving every 100 fs were performed. The fitted MSD exponents are shown along with the corresponding scaling lines. In the right panel, the diffusive behavior of DSPCs after the crossover time $\tau_c \approx 10$ ns is shown with power-law fits.

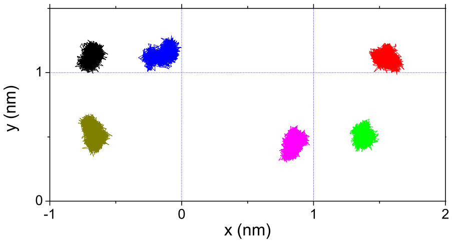


FIG. S11: DSPC sample trajectories relative to CM during simulation (100 ns) in the gel phase bilayer.

## D. Gel phase phospholipid bilayers

**(1) Trajectories of DSPCs (Fig. S11)** Compared to the liquid phase bilayer (Figs. S2 and S5) the lateral diffusivity of the lipids in the gel phase bilayer is considerably reduced. There are also no jump-like displacements of the lateral motion.

**(2) Individual TA MSDs and their scatter distribution (Fig. S12)** The TA MSDs for individual lipid molecules are sublinear and their scatter distributions are bell-shaped and centered around their averages, meaning that the lipid diffusion in the gel phase bilayer is also ergodic.

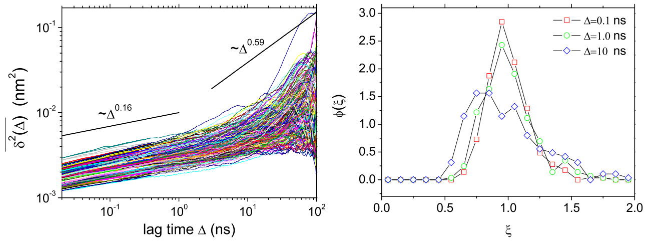


FIG. S12: Individual TA MSDs $\overline{\delta^2(\Delta)}$ of 288 DSPC molecules in the gel phase (Left) and normalized scatter distribution $\phi(\xi)$ as function of $\xi = \overline{\delta^2}/\langle\overline{\delta^2}\rangle$, at three lag times $\Delta$.(Right).

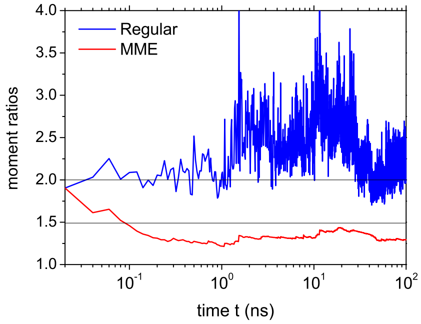


FIG. S13: Moment ratios $\langle r^4_{\max}(t)\rangle/\langle r^2_{\max}(t)\rangle^2$ (MME) and $\langle \mathbf{r}^4(t)\rangle/\langle \mathbf{r}^2(t)\rangle^2$ (regular) for DSPC lipids in the gel phase.

**(3) Moment ratios (Fig. S13)** While the regular moment ratio has a wild fluctuation around 2, the mean maximal excursion (MME) ratio saturates below 1.49. These observations are consistent with those of FLE.

### E. Rattling dynamics is of FLE type

The escape time distributions $\wp(t)$ of the rattling dynamics of lipid molecules in liquid and gel phase bilayers are displayed for several threshold radii $R$ in Fig. S14. The results are summarized as follows: (i) For both cases $\wp(t)$ is not of power-law form, as illustrated by the clear concave shape on the log-log scale in the inset. Since the escape time distribution of a CTRW process is known to follow a power-law decay [7], the result consistently supports that the anomalous diffusion of lipids is not of CTRW type. (ii) For the lipids in the liquid phase ($\alpha_s \approx 0.5 \sim 0.6$), $\wp(t)$ is clearly an exponentially decaying function. (iii) For the lipids in the gel phase ($\alpha_s \approx 0.16$), while the profiles of $\wp(t)$ are different from those for the liquid phase, the long-time tails appear to decay exponentially. We checked by simulation whether the above behaviors of $\wp(t)$ are qualitatively consistent with the corresponding distributions of FLE [8]. From the fact that the FLE in the overdamped limit (on the time scale where the lipid motion is subdiffusive) is equivalent to a fractional Brownian motion (FBM) (see Eqs. (14) and (15) for a rigorous mathematical relation between the overdamped FLE and FBM), we performed simulations of the computationally cheaper two-dimensional FBM and obtained their first escape time distributions in Fig. S15 for several threshold radii $R$ [9]. As can be seen the obtained distributions for both $\alpha = 0.14$ and $\alpha = 0.5$ are qualitatively similar to $\wp(t)$ of the lipids. The consistency of the first escape behavior in the rattling dynamics underlines our results that also in the gel phase the dynamics is of FLE type.

### F. Concerted motion of lipids

Recent numerical [4] and experimental [5] studies reported that instead of the jump-like motion the lipid molecules tend to move together, forming loosely defined local clusters with their neighbors. We identified that such concerted motion of lipids indeed occurs in our simulation. In Fig. S16 we plotted the map of the displacement vectors $\mathbf{r}(t+\delta t)-\mathbf{r}(t)$ of individual lipid molecules for given time intervals $\delta t$. Consistent with Ref. [4] the lipid displacements exhibit flow-like pattern for both $\delta t$ =1 ns and 5 ns, indicating that the lateral displacements of neighboring lipids are correlated. The observed correlations decrease quickly with $\delta t$, for $\delta t$ over 10 ns they are negligible. Note that the flow-like pattern represents the collective thermal motion of the lipids, not a real flow that would lead to ballistic motion. Concurrently, as shown in our study an *individual molecule* performs a subdiffusive motion (below the crossover time). Because of this, during the time interval measured in Fig. S16 the actual path of lateral motions of the lipids is always much longer than the magnitude of the displacement vectors. The differences between the plotted displacements and the much longer, actual path can be explained by anticorrelated motion hardwired into the FLE. Thus the overall picture is that subdiffusive lipids, with FLE as underlying subdiffusive mechanism, can simultaneously show concerted motion with their neighbors by establishing short transient clusters as shown here. In this sense, the positive correlation of lateral displacement of neighboring lipids (i.e., $\langle[\mathbf{r}_i(t+\delta t)-\mathbf{r}_i(t)]\cdot[\mathbf{r}_j(t+\delta t)-\mathbf{r}_j(t)]\rangle$ with the lipid index $i\neq j$) does not contradict our findings in this paper, i.e., FLE-like subdiffusive motion of a lipid molecule and its negative autocorrelation $\langle[\mathbf{r}_i(t+\delta t)-\mathbf{r}_i(t)]\cdot[\mathbf{r}_i(\delta t)-\mathbf{r}_i(0)]\rangle$.

### G. Change of neighbors and mixing

One of the immediate consequences of the diffusion process in membranes is the change of any given lipid with one of its neighbors. Although several mechanisms exist which explain the change of neighbors (flow, change, vacuum jumps ...) the result is always the same, namely mixing, and in our case a memory loss from the artificial initial configuration. To complete the membrane dynamics study offered in this work we have also quantified the change of neighbors in the simulated membranes, see Fig. S17.

The method developed requires the definition of two radii around the center of mass of the analyzed lipid. The first one is chosen to be small enough so that if any other lipid (center of mass) is found within its borders it is surely in direct contact. The second radius, in contrast, is chosen to be large enough so that any lipid (center of mass) outside its border can be safely considered as not being in contact. Using the in-plane radial distribution

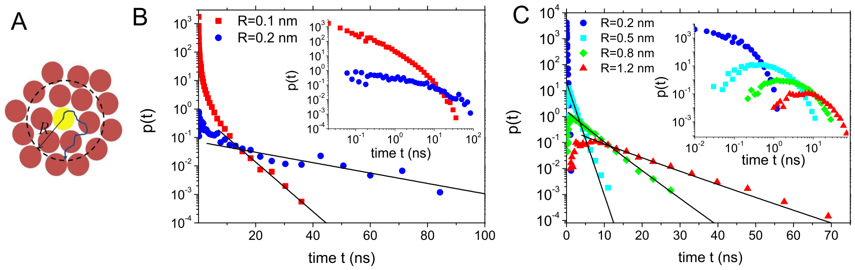


FIG. S14: A. Schematic showing the rattling dynamics of lipid molecules and the definition of their first escape event. Here the first escape time of a tracer lipid molecule (yellow circle) is defined by the moment that its radial displacement from the initial position, for the first time, crosses a threshold value denoted by $R$. B. The corresponding first escape time density $\wp(t)$ of the DSPC molecules in pure gel phase bilayer for different values of the threshold radius $R$. C. First escape time density $\wp(t)$ of the DSPC molecules in pure liquid phase bilayer. In B and C the black lines are the exponential fitting. The insets show the same data on a double-logarithmic scale. The behavior is fully consistent with simulations results of FBM shown in Fig. S15.

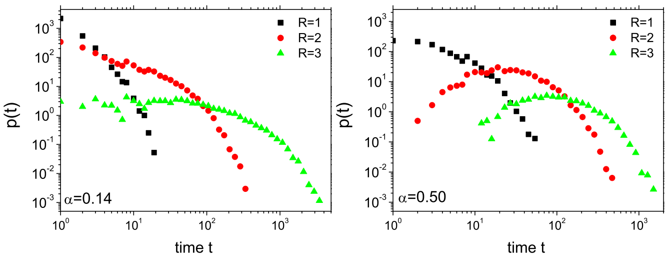


FIG. S15: First escape time distribution of two-dimensional FBM for $\alpha = 0.14$ (Left) and $\alpha = 0.5$ (Right).

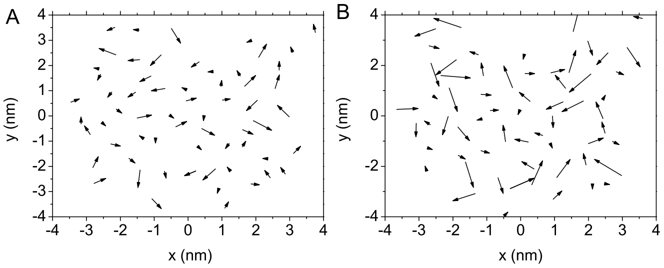


FIG. S16: Displacement vectors $\mathbf{r}(t + \delta t) - \mathbf{r}(t)$ of all DSPC molecules during time interval $\delta t$ in the upper layer of the pure bilayers for (A) $\delta t$ =1 ns and $t$ = 1 ns, and (B) $\delta t$ = 5 ns and $t$ = 5 ns.

functions between the center of mass of the phospholipids and cholesterols [11] we have chosen them as 0.6 nm and 1.6 nm. These values are really restrictive to guarantee the contact and non-contact criteria. Once the radii are defined, for a given time/frame, a list of contact pairs (distance < 0.6 nm) is calculated. Our restrictive radius on average provides less than one lipid in contact per lipid (128 pure/160 Mix-cholesterol membranes), see Fig. S17. For later times we check how many of the initial contacts are still in place (distance < 1.6 nm), and we register their number. This analysis is repeated every 10 ns using the corresponding frame to construct the list and the following frames to study the decay of the contacts. It is important to mention that the small size of our systems, $6{\times}6$ nm$^2$ in the membrane plane, makes it relatively easy for a detached lipid to come back to the contact region (sphere of 3.2 nm diameter around a lipid). This fact, in addition to the large escape radius chosen, provide an underestimated measure of the real change of neighbors along the simulation which one can expect to be larger.

Fig. S17 shows, respectively, the decay of neighbor contacts for the pure DSPC membrane pure and mixed with cholesterol by using the method described above. In both cases a clear decay is observed. The DSPC gel phase membrane on the contrary does not show any decay (not shown). Notice that after 100 ns for pure DSPC membrane the contact curve reaches a plateau at around 20% of the initial contacts. The plateau is a consequence of the small lateral dimensions of our membranes. For bigger systems the curves are expected to decay to zero. For a membrane containing cholesterol we observe a smaller rate of change of neighbors yet it is sufficient to ensure the mixing in the time scale of the presented simulations. SOPC and DOPC membranes possess significantly higher rates of change of neighbors corresponding to their higher diffusion rates.

Finally, visual inspection of the trajectories of the center of mass of the lipids clearly shows that the change of neighbors characterized here occurs via flow and neither by jumps nor cooperative change of lipids.

### H. Two-dimensional liquid Argon system

We simulated a 2D liquid Argon as an additional control. A three-dimensional system consisting of 10,800 Argon atoms was first simulated at its boiling point (87.3 K), and the experimental density was reproduced at 1 atm [12]. Then, a two-dimensional system of 9,000 Argon atoms was simulated and the lateral pressure was varied until the diffusion coefficient agreed with that of the 3D system. The results are plotted in Fig. S18. The

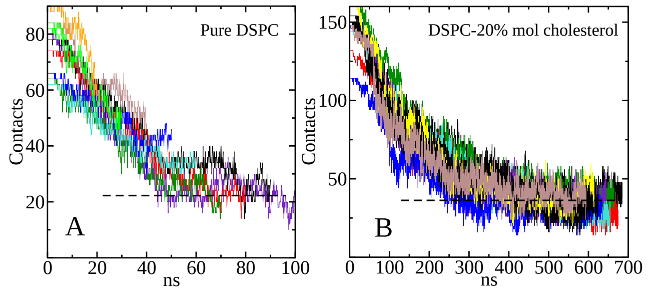


FIG. S17: Decay of contacts as function of time for (a) pure DSPC membrane and (b) DSPC – 20% mol cholesterol membrane. Different curves corresponding to different initial times are plotted for each system. All curves show similar decay behavior of contacts. The rate of decay is inversely proportional to the change of neighbors rates. The black dashed line shows the plateau due to the small in-plane size of the membrane that makes it likely for a destroyed contact to be formed again after some time.

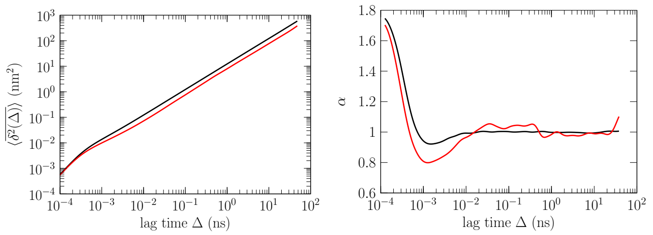


FIG. S18: (Left) Averaged TA MSD $\langle\overline{\delta^2(\Delta)}\rangle$ over all Argon atoms in 2D (red) and 3D (black) space. (Right) The variation of the corresponding MSD exponent $\alpha$ for the TA MSDs as function of lag time.

MSD curves show ballistic motion at short times and a very short subdiffusion region (from subpicosecond to a few picoseconds) with a subdiffusion exponent of about 0.8. The qualitative behavior of 2D and 3D systems is similar yet the subdiffusion exponent is smaller in the 2D system. Decrease in temperature resulted in smaller subdiffusion exponents yet the time region of anomalous diffusion remained similar. Notably, the transition from the subdiffusion regime to normal diffusion occurs fast within a few dozen picoseconds. This is in close agreement with the characteristic time required for an argon atom to diffuse a distance equal to its diameter, namely 14 ps.

## II. SIMULATIONS

We carried out atomic-scale molecular dynamics (MD) simulations for seven different membrane systems, modeling the different membrane phases: liquid disordered ($L_\alpha$), liquid ordered ($L_o$), and gel ($L_\beta$), see Fig. 1.

The first three systems correspond to pure membranes constituted by 128 phosphatidylcholines with 18 carbon chains (non-raft). These three systems just differ in the degree of unsaturation of their constituent lipids. While the first membrane is composed of high melting point DSPC lipids (two saturated stearoyl chains), the second contains low melting point DOPC lipids (two cis-monounsaturated oleoyl chains). The third membrane is constituted of SOPC lipids (*sn*-1 stearoyl and *sn*-2 oleoyl chains) whose properties range in between DSPC and DOPC lipids. As expected from the simulation temperature 338 K the typical behavior of the $L_\alpha$ phase is observed in all these membranes. The selected temperature is above the main phase transition temperature of DSPC ($T_m$ = 328 K), the highest among the studied lipid species [10]. All three membranes are often used in comparative experimental and theoretical studies due to their distinctive behavior and properties. In particular, their area per molecule increases with the number of unsaturated chains and therefore the molecular disorder [13].

The next three systems correspond to the same pure membranes considered above, in addition to which 32 cholesterol molecules were included (corresponding to 20% mol) at 338 K. The role of cholesterol in biological membranes is outstanding [14]. One important property pertaining to this work is that the presence of cholesterol induces a new phase, the $L_o$ phase, especially when mixed with high melting point lipids. The $L_o$ phase is still rather liquid but the bilayer becomes more rigid, more ordered, thicker, and less permeable. In our simulations all these changes are clearly visible when mixing cholesterol with DSPC, see Fig. 1. Instead, mixing with DOPC does not change much the behavior found in the pure membranes, while with SOPC the results are again intermediate.

These six systems were fully hydrated by adding 31 water molecules per lipid. We used the standard united-atom Berger force field parameters that have been extensively tested [13, 15, 16]. The partial charges were taken from the underlying model description [16]. For the double bond, we employed the approach by Bachar et al. [17]. The Simple Point Charge (SPC) model [18] was used for water. For cholesterol, we followed Holtje et al. [19].

To get an overall picture we also simulated DSPC at 310 K. At this temperature DSPC is in its gel phase. Our simulations of DSPC with the Berger-lipids force field at this temperature showed that the membrane is still in the liquid disordered phase. To solve this we used an OPLS all atom DSPC membrane whose phase behavior is correct at 310 K [20]. Employing a different force field poses no problem, but instead it makes our results more robust as both force fields produce the same dynamic behavior. In this gel phase membrane the number of DSPC lipids was 288. The number of water molecules per lipid was 44, and 31 NaCl ions were added, some of which are visible in the water phase in Fig. 1.

All simulations were performed using the GROMACS package [21], in the $NpT$ ensemble at $p = 1$ atm. Temperature and pressure were controlled by using the weak

coupling method [22] with the respective relaxation times set to 0.6 and 1.0 ps. The temperatures of the solute and solvent were controlled independently, and the pressure coupling was applied separately in the bilayer plane and normal to it. A single cutoff distance 1.0 nm was used for the Lennard-Jones interactions [23]. The long-range electrostatic interactions were handled using the particle-mesh Ewald method [23], with a real space cutoff of 1.0 nm, sixth order spline interpolation, and direct sum tolerance of $10^{-5}$. All interactions lists were updated at each time step. The system's center of mass movement was removed at every time step. The SETTLE algorithm [24] was used to preserve the bond lengths of the water molecules, whereas the lipid bond lengths were constrained by the LINCS algorithm [25]. Periodic boundary conditions with the usual minimum image convention were used in all three directions, and the time step was set to 2 fs. Each pure system was run for 100 ns after 20 ns equilibration, and each membrane containing cholesterol for 150 ns after 20 ns equilibration. In both cases all systems were previously run for at least 300 ns ensuring no memory from the initial conditions, see Section I.G. The gel phase system was run for 100 ns after 100 ns equilibration. For a more detailed description of the initial setup and the resulting structural and dynamic properties see Refs. [13, 20, 26, 27].

## III. DISPLACEMENT AUTOCORRELATION

In the main text the displacement autocorrelation function over a time interval $\delta t$ is defined as

$$C_{\delta t}(t) = \frac{1}{\delta t^2}\langle[\mathbf{r}(t+\delta t) - \mathbf{r}(t)]\cdot[\mathbf{r}(\delta t) - \mathbf{r}(0)]\rangle, \quad (1)$$

where $\mathbf{r}(t)$ is the 2D vector of the lipid position relative to CM. The displacement autocorrelators for CTRW and FBM in free space were derived in Ref. [28], resulting in

$$\frac{C_{\delta t}(t)}{C_{\delta t}(0)} = \begin{cases} 1-(t/\delta t)^\alpha & t \le \delta t \\ 0 & t \ge \delta t \end{cases}, \quad (2)$$

for free CTRW motion, due to the statistical independence of successive jump events. Free FBM (or overdamped FLE motion) has the autocorrelator

$$\frac{C_{\delta t}(t)}{C_{\delta t}(0)} = \frac{|t+\delta t|^\alpha - 2t^\alpha + |t-\delta t|^\alpha}{2\delta t^\alpha}. \quad (3)$$

The FLE describes ergodic anomalous diffusion and fulfills the fluctuation-dissipation theorem. In free 1D space, a particle of mass $m$ and generalized friction $\gamma$ following FLE motion $x_\alpha(t)$ is described by

$$m\frac{d^2x_\alpha(t)}{dt^2} = -\gamma\int_0^t dt'|t-t'|^{-\alpha}\frac{dx_\alpha}{dt'} + \eta\xi(t). \quad (4)$$

Here the index $\alpha < 1$ stands for the scaling exponent of its MSD in the overdamped limit as explained below. In the framework of the FLE, the thermal noise $\xi(t)$ is persistent fractional Gaussian noise with $\langle\xi(t)\rangle = 0$ and $\langle\xi(t)\xi(t')\rangle = (2-\alpha)(1-\alpha)K_\alpha|t-t'|^{-\alpha}$ at $t \neq t'$, and $\eta = \sqrt{\gamma/[(2-\alpha)(1-\alpha)\beta K_\alpha]}$. The initial condition is $x_\alpha(0) = 0$, and the velocity $dx_\alpha(0)/dt \equiv v_0$ follows the Boltzmann distribution, with the MSD

$$\langle x_\alpha^2(t)\rangle = \frac{2t^2}{\beta m}E_{2-\alpha,3}\left[-\Gamma(1-\alpha)\frac{\gamma}{m}t^{2-\alpha}\right], \quad (5)$$

where $E_{a,b}(z)$ is the generalized Mittag-Leffler function with series expansions around $z = 0$ and $z \to \infty$,

$$E_{a,b}(z) = \sum_{n=0}^{\infty}\frac{z^n}{\Gamma(a+bn)} = -\sum_{n=1}^{\infty}\frac{z^{-n}}{\Gamma(b-an)}. \quad (6)$$

The MSD turns from short-time ballistic motion $\langle x_\alpha^2(t)\rangle \sim t^2$ to subdiffusive motion $\langle x_\alpha^2(t)\rangle \sim t^\alpha$.

To calculate the displacement autocorrelation function above, one needs the covariance of the position, $\langle x_\alpha(t_1)x_\alpha(t_2)\rangle$. For FLE motion in free space,

$$\begin{aligned}\langle x_\alpha(t_1)x_\alpha(t_2)\rangle = \frac{k_BT}{m}\Big[&t_1^2E_{2-\alpha,3}(-\zeta t_1^{2-\alpha}) \\ &+t_2^2E_{2-\alpha,3}(-\zeta t_2^{2-\alpha}) \\ &-(t_2-t_1)^2E_{2-\alpha,3}(-\zeta|t_2-t_1|^{2-\alpha})\Big], \quad (7)\end{aligned}$$

where $\zeta = \Gamma(1-\alpha)\gamma/m$. Using this we obtain the analytic form of the autocorrelation function

$$\frac{C_{\delta t}(t)}{C_{\delta t}(0)} = \frac{\mathcal{F}(t+\delta t) + \mathcal{F}(|t-\delta t|) - 2\mathcal{F}(t)}{2\mathcal{F}(\delta t)} \quad (8)$$

for $t > 0$, where $\mathcal{F}(x) = x^2E_{2-\alpha,3}(-\zeta x^{2-\alpha})$. In the main text, $\delta t$ was set to be 0.2 ns. On this timescale, the motion belongs to the regime of subdiffusion. In this overdamped limit the above form is simplified to

$$\frac{C_{\delta t}(t)}{C_{\delta t}(0)} = \frac{(t+\delta t)^\alpha - 2t^\alpha + |t-\delta t|^\alpha}{2\delta t^\alpha}. \quad (9)$$

Interestingly this functional form in the overdamped limit of FLE motion is identical with that of FBM, meaning that the FLE in the overdamped limit has the same statistical property of spatial movements as FBM. Note that there is no free parameter in $C_{\delta t}(t)/C_{\delta t}(0)$. In the main text we compare Eq. (9) with the simulations result $C_{\delta t}(t)/C_{\delta t}(0)$ of lipids, where the value of $\alpha$ was estimated from the time averaged MSD.

## IV. MOMENT RATIOS

Here we mathematically derive the moment ratios, $\langle\mathbf{r}^4(t)\rangle/\langle\mathbf{r}^2(t)\rangle^2$ and $\langle r_{\max}^4(t)\rangle/\langle r_{\max}^2(t)\rangle^2$, for two-dimensional FLE motion. The cases of CTRW and FBM were discussed in Ref. [29]: free CTRW ($0 < \alpha < 1$) has the moment ratios $\langle\mathbf{r}^4(t)\rangle/\langle\mathbf{r}^2(t)\rangle^2 > 2$

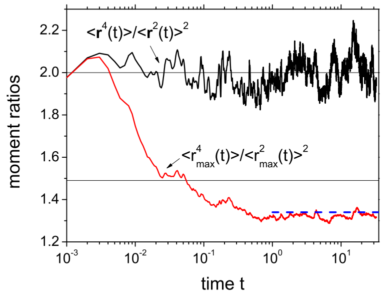


FIG. S19: Moment ratios of FLE motion obtained from simulations. Parameter values used in the simulations are: unit mass $m = 1$, generalized frictional coefficient $\gamma = 1000$, normalized Boltzmann factor $k_BT = 1$, anomalous diffusion exponent $\alpha = 0.7$, and time step 0.001. The two solid lines represent the theoretical values $\langle \mathbf{r}^4(t)\rangle/\langle \mathbf{r}^2(t)\rangle^2 = 2$ and $\langle r^4_{\max}(t)\rangle/\langle r^2_{\max}(t)\rangle^2 < 1.49$ in the overdamped limit. The dashed line is the expected value $\approx 1.34$ of $\langle r^4_{\max}(t)\rangle/\langle r^2_{\max}(t)\rangle^2$ for the given value $\alpha = 0.70$.

and $\langle r^4_{\max}(t)\rangle/\langle r^2_{\max}(t)\rangle^2 > 1.49$. The behavior for free subdiffusive FBM is $\langle \mathbf{r}^4(t)\rangle/\langle \mathbf{r}^2(t)\rangle^2 = 2$ and $\langle r^4_{\max}(t)\rangle/\langle r^2_{\max}(t)\rangle^2 < 1.49$.

**(1) Moment ratios in the ballistic regime**

Although in the ballistic regime the motion is deterministic, such that $x_\alpha(t) = v_0 t$, the moments of the position $x_\alpha(t)$ have a non-sharp distribution as the velocity $v_0$ is a random variable. If we decompose the 2D motion described by the FLE in terms of $\mathbf{r}(t) = (x_\alpha(t), y_\alpha(t))$, the second and fourth moments of each component $x_\alpha(t)$ are

$$\langle x^2_\alpha(t)\rangle = \langle v^2\rangle_{th} t^2 = (k_BT/m)t^2, \quad (10)$$
$$\langle x^4_\alpha(t)\rangle = \langle v^4\rangle_{th} t^4 = 3\,(k_BT/m)^2\, t^4, \quad (11)$$

where $\langle\cdot\rangle_{th}$ denotes the thermal average. From these relations, we find the regular moment ratio

$$\frac{\langle \mathbf{r}^4(t)\rangle}{\langle \mathbf{r}^2(t)\rangle^2} = \frac{\langle x^4_\alpha(t)\rangle + \langle y^4_\alpha(t)\rangle + 2\langle x^2_\alpha(t)\rangle\langle y^2_\alpha(t)\rangle}{(\langle x^2_\alpha(t)\rangle + \langle y^2_\alpha(t)\rangle)^2} = 2. \quad (12)$$

In the ballistic regime $x_{\max}(t) = x(t)$ as $x(t) = v_0 t$. Thus $\langle x^2(t)\rangle = \langle x^2_{\max}(t)\rangle$ and $\langle x^4(t)\rangle = \langle x^4_{\max}(t)\rangle$. The MME moment ratio is the same as that of the regular moments:

$$\langle r^4_{\max}(t)\rangle/\langle r^2_{\max}(t)\rangle^2 = 2. \quad (13)$$

**(2) Moment ratios in the Brownian limit**

In the limit $\alpha = 1$, the above FLE reduces to the ordinary Langevin equation with white, Gaussian noise. Beyond the ballistic regime, the FLE in the overdamped limit corresponds to ordinary Brownian motion. In this case, the exact analytical values of the moment ratios are (see Ref. [29]) $\langle \mathbf{r}^4(t)\rangle/\langle \mathbf{r}^2(t)\rangle^2 = 2$ and 1.49 ($\langle r^4_{\max}(t)\rangle/\langle r^2_{\max}(t)\rangle^2 \cong 1.49$) for 2D motion.

**(3) Moment ratios in the subdiffusive regime**

As shown by Deng and Barkai [30], in the overdamped limit the above equation (4) can be rewritten as

$$x_\alpha(t) = \frac{\eta}{\gamma\Gamma(1-\alpha)}\, {}_0D_t^{-\alpha}\xi(t), \quad (14)$$

where ${}_0D_t^{-\alpha}$ is the Riemann–Liouville fractional integral of order $\alpha$ [31]. From this relation, it was shown that

$$\langle x_\alpha(t)\rangle = 0, \quad \langle x_\alpha(t_1)x_\alpha(t_2)\rangle = K_F(t_1^\alpha + t_2^\alpha - |t_1 - t_2|^\alpha) \quad (15)$$

where $K_F$ depends on temperature, friction $\gamma$, and $\alpha$. Thus $x_\alpha(t)$ in the overdamped limit is an FBM, its MSD growing like $\langle x^2_\alpha(t)\rangle = 2K_F t^\alpha$. Accordingly, overdamped FLE motion has the same moment ratios as FBM:

$$\langle \mathbf{r}^4(t)\rangle/\langle \mathbf{r}^2(t)\rangle^2 = 2 \quad (16)$$
$$\langle r^4_{\max}(t)\rangle/\langle r^2_{\max}(t)\rangle^2 \cong 1.05(\alpha/2)^{1.42} + 1.10, \quad (17)$$

as $t \to \infty$ (see Ref. [29] for the mathematical derivation of the ratios). Thus for FLE motion with $\alpha < 1$ the moment ratio of the mean maximal excursion fulfills the criterion

$$\langle r^4_{\max}(t)\rangle/\langle r^2_{\max}(t)\rangle^2 < 1.49. \quad (18)$$

**(4) Comparison with simulations**

Fig. S19 shows the moment ratios of two-dimensional FLE motion obtained from simulation of 1000 runs, along with the theoretical values discussed above. In the simulations we chose $\alpha = 0.70$. The regular moment ratio fluctuates around the theoretical value $\langle \mathbf{r}^4(t)\rangle/\langle \mathbf{r}^2(t)\rangle^2 = 2$ (solid line) at all times. For the moment ratio of the mean maximal excursion (MME), as predicted from theory, $\langle r^4_{\max}(t)\rangle/\langle r^2_{\max}(t)\rangle^2$ is around 2 in the ballistic regime and decreases to a value below 1.49 (the crossover value) in the overdamped limit. It is also shown that the asymptotic value approaches the corresponding theoretical value $\langle r^4_{\max}(t)\rangle/\langle r^2_{\max}(t)\rangle^2 \approx 1.34$ (dotted line) for the given value of $\alpha$.


[1] T. Akimoto et al., Phys. Rev. Lett. **107**, 178103 (2011).
[2] C. Hofsäß, E. Lindahl, and O. Edholm, Biophys. J. **84**, 2192 (2003).
[3] J. D. Perlmutter, and J. N. Sachs, J. Am. Chem. Soc. **133**, 6563 (2011).
[4] E. Falck, T. Rog, M. Karttunen, and I. Vattulainen, J. Am. Chem. Soc. **130**, 44 (2008).
[5] S. Busch, C. Smuda, L. C. Pardo, and T. Unruh, J. Am. Chem. Soc. **132**, 3232 (2010).
[6] E. Flenner et al., Phys. Rev. E **79**, 011907 (2009).
[7] R. Metzler and J. Klafter, J. Phys. A **37**, R161 (2004).
[8] The statistical behaviors of the escape time distribution

(i.e., the first passage time distribution in finite domain) of FLE is not rarely studied.
[9] When the length of simulation is long, the simulation of FBM is much faster than that of FLE. To acquire statistically reliable long-time tail of the first escape time distribution, we simulated FBM with the exponent $\alpha$ corresponding to $\alpha_s$ for the liquid and gel phases found in MD simulation.
[10] R. Koyanova and M. Caffrey, Biochim. Biophys. Acta **1376**, 91 (1998).
[11] H. Martinez-Seara et al., PLoS One **5**, e11162 (2010).
[12] L. A Rowley, D. Nicholson, and N. G Parsonage, J. Comp. Phys. **17**, 401 (1975).
[13] H. Martinez-Seara, T. Rog, M. Pasenkiewicz-Gierula, I. Vattulainen, M. Karttunen, and R. Reigada, J. Phys. Chem. B **111**, 11162 (2007).
[14] D. Lingwood and K. Simons, Science **327**, 46 (2010).
[15] O. Berger, O. Edholm, and F. Jahnig, Biophys. J. **72** 2002 (1997).
[16] D. P. Tieleman and H. J. C. Berendsen, J. Chem. Phys. **105**, 4871 (1996).
[17] M. Bachar, P. Brunelle, D. P. Tieleman, and A. Rauk, J. Phys. Chem. B **108**, 7170 (2004).
[18] H. J. C. Berendsen, J. P. M. Postma, W. F. van Gunsteren, and J. Hermans, in *Intermolecular Forces*, eds Pullman (Reidel, Dordrecht, 1981), pp 331-342.
[19] M. Holtje, T. Forster, B. Brandt, T. Engels, W. von Rybinski, and H. D. Holtje, Biochim. Biophys. Acta, **1511**, 156 (2001).
[20] M. Stepniewski, A. Bunker, M. Pasenkiewicz-Gierula, M. Karttunen, and T. Rog, J. Phys. Chem. B **114**, 11784 (2010).
[21] E. Lindahl, B. Hess, D. van der Spoel, J. Mol. Model. **7**, 306 (2001).
[22] H. J. C Berendsen, J. P. M. Postma, W. F. van Gunsteren, A. DiNola, and J. R. Haak, J. Chem. Phys. **81**, 3684 (1984).
[23] U. Essman, L. Perera, M. L. Berkowitz, H. L. T. Darden, and L. G. Pedersen, J. Chem. Phys. **103**, 8577 (1995).
[24] S. Miyamoto and P. A. Kollman, J. Comp. Chem. **13**, 952 (1992).
[25] B. Hess, H. Bekker, H. J. C. Berendsen, and J. G. E. M. Fraaije, J. Comp. Chem. **18**, 1463 (1997).
[26] H. Martinez-Seara, T. Rog, M. Karttunen, I. Vattulainen, and R. Reigada, J. Phys. Chem. B **113**, 8347 (2009).
[27] H. Martinez-Seara, T. Rog, M. Pasenkiewicz-Gierula, I. Vattulainen, M. Karttunen, and R. Reigada, Biophys. J. **95**, 3295 (2008).
[28] S. Burov, J.-H. Jeon, R. Metzler, and E. Barkai, Phys. Chem. Chem. Phys. **13**, 1800 (2011).
[29] V. Tejedor et al., Biophys. J. **98**, 1364 (2010).
[30] W. Deng and E. Barkai, Phys. Rev. E. **79**, 011112 (2009).
[31] R. Metzler and J. Klafter, Phys. Rep. **339**, 1 (2000).
